# Supplementary material for: Combining LLMs with Logic-Based Framework to Explain MCTS
Source: arXiv:2505.00610 source file (2025-05-01)
Supplement: Supplementary file 1 [file 6_supp.tex]

\clearpage
\FloatBarrier
\begin{figure*}[t]
\centering
  \includegraphics[width=\linewidth]{figs/Screenshot 2024-10-01 at 7.17.52 PM.png}
  \caption{LogiEx Chatbot Interface.}
  \label{fig:interface}
\end{figure*}

\section{Appendix}

\subsection{LogiEx Scorer Algorithm}
\begin{algorithm}[H]
\small
\caption{\small \textit{LogiEx} Variable Scorer}
\label{alg:expgen}
    \begin{flushleft}
    \begin{algorithmic}[1]
    \STATE \textbf{Input:} Variables $\mathcal{X}$, $\mathcal{V}$, $\Phi$, scorer functions $f, g$
    \STATE \textbf{Output:} Extracted evidence results $evi$
    \STATE Initialize evidence results $evi \leftarrow \{\}$
    \\ \texttt{/* obtain result for base-level evidence */} 
    \FOR{each base-level variable $X_i \in \mathcal{X}$} 
        \STATE Compute and store $f_i(X_i)$ in $evi$
    \ENDFOR
    \\ \texttt{/* obtain result for second-level evidence */} 
    \FOR{each derived variable $V_j \in \mathcal{V}$} 
        \FOR{each relevant child state $s$ in the MCTS tree} 
            \IF{$V_j$ depends on base-level variable $X_j$}
                \STATE Compute $f_j(X_j)$ and store as temporary result
            \ENDIF
            \STATE Evaluate and store $g_j(V_j)$ in $evi$
        \ENDFOR
    \ENDFOR
    \\ \texttt{/* obtain result for logic comparison evidence */} 
    \FOR{each logic comparison variable $\Phi_k \in \Phi$} 
        \FOR{each relevant child state $s$ in the MCTS tree} 
            \IF{$\Phi_k$ depends on base-level variable $V_k$}
            \IF{$V_k$ depends on derived variable $X_k$}
            \STATE Compute $f_k(X_k)$ and store as temporary result
            \ENDIF
                \STATE Compute $g_k(V_k)$ store as temporary result
            \ENDIF
            \STATE Evaluate logical condition $P(s) \implies \Phi_k$ and store result in $evi$
        \ENDFOR
    \ENDFOR
    
    \STATE \textbf{Return} evidence results $evi$
    \end{algorithmic}
    \end{flushleft}
\end{algorithm}

\subsection{Reward Function}

The reward function is calculated as a weighted sum of two components: the first part, $w_f$, represents the trip fulfillment ratio, and the second part, $w_t$, accounts for the timing difference between the scheduled and actual times. Let $R$ be the set of trip requests, and $|R|$ is the total number of requests. For the trip fulfillment component, all requests with a status of ``in-transit'' or ``dropped-off'' are considered fulfilled. Thus, the trip fulfillment ratio is calculated as the following, where $\varmathbb{1}$ is the indicator function:
\[
w_{f} = \frac{1}{|R|} \sum_{i=1}^{|R|} \varmathbb{1}\left( u_i = \text{``in-transit''} \text{ or } \text{``dropped-off''} \right)
\]

For each request $i \in R$, $t_{ap}^i$ is the actual pick-up time, and $t_{ad}^i$ is the actual drop-off time, which may be different from the requested times. To calculate the timing component of the reward, we consider the difference between the specified times and the actual times for each trip \( i \). Specifically, if the status is ``in-transit'': $
\text{ Timing}_i = t_{ap}^i - t_p^i$. And if the status is ``dropped-off'': $
\text{Timing}_i = (t_d^i - t_{ad}^i ) + (t_{ap}^i - t_p^i)$. 
The total timing component for all trips is therefore: 
\[w_{t} = \sum_{i=1}^{|R|} \text{Timing}_i\]

Let the $a$ and $b$ be the weights for trip fulfillment and timing components respectively. The final reward function is a linear combination of the two components: \[\text{Reward} = a \cdot w_{f} + b \cdot w_{t}\]

\subsection{Additional Information on RAG}
The proposed RAG method follows a process that includes \textbf{Indexing}, \textbf{Retrieval}, and \textbf{Generation}. During indexing, the knowledge base is prepared in a plain text format, segmented into smaller chunks to accommodate the context limitations of LLMs. These chunks are encoded into vector representations using the embedding model of \textit{text-embedding-3-small}, one of the newest and most performant embedding models provided by OpenAI, and stored in a vector database. In the retrieval phase, the RAG system transforms the user query into a vector representation, computes \textit{cosine similarity} scores between the query and the vectorized chunks, and retrieves the top $K$ most relevant chunks. These chunks are then used as expanded context in the generation phase, where the query and selected documents are synthesized into a comprehensive prompt, empowering LLMs to generate well-informed answers.

Providing explanations about MCTS-based transit routing suggestions is a domain-specific and knowledge-intensive task. We expect the LLM agent to act as a domain expert, delivering accurate and credible answers, thereby increasing user satisfaction. To achieve this, we leverage the advanced capabilities of RAG, which merges the intrinsic knowledge of LLMs with dynamic repositories of external databases, such as a knowledge base aligned with this specific use case.

To avoid information overload, it is essential to select only the critical information, emphasize important sections, and shorten the context processed by the LLMs. For this work, we prepared a knowledge base containing approximately 3000 words, divided into 34 chunks. This knowledge base covers background information on the paratransit service and the MCTS algorithm, detailed components of the proposed MCTS system, including predefined constraints, algorithm objectives, the encapsulated reward function used for decision-making, and expert-generated queries and answers. 

RAG's cost-effectiveness and its ability to surpass native LLM performance make it an ideal solution for providing enhanced information to LLM agents, enabling them to handle more complex and knowledge-intensive tasks. RAG operates through three core components: \textbf{Retrieval}, \textbf{Augmentation}, and \textbf{Generation}\cite{gao2023retrieval}. During the retrieval phase, RAG fetches relevant document chunks from external databases based on the semantic similarity to the user query. In the augmentation phase, the retrieved information is integrated into the in-context learning process, allowing continuous updates and better handling of domain-specific data. Finally, during the generation phase, LLMs synthesize the augmented information into coherent answers.

\subsection{Knowledge Base Topics}
\begin{itemize}
    \item \textbf{Paratransit Introduction}: Paratransit services operate within the same areas and hours as fixed-route systems and provide curb-to-curb transportation, using a fleet of vehicles on an on-demand basis, i.e., the service considers user requests as they are made.
    \item \textbf{Service Rules}: Passengers must provide pickup instructions, including the Origin (O), Destination (D), and expected pick-up and drop-off time.
    \item \textbf{Vehicle Assignment Algorithm (MCTS)}: The MCTS algorithm optimizes vehicle assignments by considering factors such as seating capacity, pickup/drop-off time, and overall route efficiency. The goal is to accommodate as many trips as possible while minimizing passenger onboard time and ensuring realistic scheduling.
    \item \textbf{Scoring and Constraints}: The algorithm assigns a composite reward score to each route, considering factors like timing adherence and future trip capacity. If all vehicle options violate constraints, such as overcapacity, the request is rejected.
    \item \textbf{Real-Time and Future Scenario Planning}: Vehicle assignments are planned in real-time as new requests arrive. The MCTS algorithm simulates multiple future scenarios to determine optimal vehicle assignments, minimizing delays and improving service efficiency. Also, the algorithm balances thorough scenario exploration with computational efficiency.
    \item \textbf{Passenger Considerations}: Early drop-offs may pose safety risks or cause inconvenience, especially if the destination is not yet open. Passengers can schedule pickups in advance, and human dispatchers monitor potential errors in the algorithm's decisions.
    \item \textbf{Human Dispatcher Role}: Human dispatchers have the final authority and can override algorithmic decisions based on real-world factors like traffic conditions or passenger needs. 
\end{itemize}

\subsection{Example Factual Information}
\begin{itemize}
    \item ``This equivalent service (ADA paratransit) is provided to persons who, because of their disabilities, are unable to independently ride a bus. ADA paratransit must be provided within the same geographic service area and during the same service hours as fixed-route bus service. The maximum fare a public transportation provider can charge for standard ADA paratransit service is twice the adult one-way bus fare. ''
    \item ``The Monte Carlo Tree Search (MCTS) algorithm on our backend assigns a vehicle to a passenger, and the vehicle assignment must adhere to the following constraints: - First, the number of assigned passengers must align with the vehicle's seating capacity, ensuring that each passenger has an allocated seat. - Second, pickup and drop-off times should be realistic, not significantly exceeding the expected duration.'' 
    \item ``How will the route be planned if there are multiple passengers? We use the MCTS algorithm to conduct the route planning task. In the current scenario, each request involves only one passenger, and there will be only one request at any given time.''
    \item ``How would we know there is an error if it’s only computer processing? Real human dispatchers are responsible for making the final vehicle assignments and overseeing the entire process. While the computer algorithm provides recommendations, human dispatchers review these suggestions and have the authority to override them at any time. This oversight allows human dispatchers to identify and correct any errors the algorithm might make, ensuring that decisions are accurate and reliable. By combining algorithmic efficiency with human judgment, we can maintain high standards of service and promptly address any issues that arise.'' 
    \item ``Why is getting dropped off early a bad thing? Isn’t an early drop-off time more desired by the passenger? Safety Concerns: Passengers, especially those with disabilities, might be dropped off in locations where it is not safe to wait for long periods.  Inconvenience: If a passenger is dropped off early, they may have to wait outside the destination, such as a doctor's office, which may not be open yet or may not allow early arrivals inside Scheduled Appointments: Many passengers use paratransit services to get to scheduled appointments (e.g., medical appointments, therapy sessions). Arriving too early can result in long waiting times, which can be physically and mentally taxing, particularly for those who have strict schedules or multiple appointments in a day. Assistance Availability: Passengers who require assistance may not have access to their companions or personal care assistants (PCAs) if they arrive earlier than expected. This can leave them without the necessary support they need until the scheduled time of their appointment or the arrival of their assistant. Personal Schedule Disruption: Passengers often plan their personal schedules around their transportation and appointment times. Arriving too early can disrupt their entire day, causing them to miss other planned activities or events.''
\end{itemize}

\subsection{Query Types and Corresponding Logic Formula}

\paragraph{Category 1}
\begin{enumerate}
    \item ``Can you tell me the scheduled pick-up time for the passenger?''; 
    \[ tp(0) \]
    \item ``Could you tell me when the passenger is scheduled to be dropped off?''; 
    \[ td(0) \]
    \item ``Can you provide the current passenger count for vehicle 1?''; 
    \[ O(0,1) \]
    \item ``What is the remaining passenger capacity of vehicle 2?''; 
    \[ vcvq(C(2), O(1,2)) \]
    \item ``What is the number of stops a passenger will face when traveling in vehicle 1?''; 
    \[ sp(0,1); sd(0,1) \]
    \item ``Could you indicate the expected arrival time for the passenger if they're assigned to vehicle 1?''; 
    \[ eta(1) \]
    \item ``Could you let me know the likely delay duration in the pick-up time for a passenger assigned to vehicle 3?''; 
    \[ viod(tp(3), eta(3)) \]
    \item ``Could you let me know the likely delay duration in the drop-off time for a passenger assigned to vehicle 3?''; 
    \[ viod(td(3), eta(3)) \]
    \item ``Could you clarify the expected time of advancement in the pick-up time for a passenger when they are assigned to vehicle 3?''; 
    \[ vioa(tp(3), eta(3)) \]
    \item ``Could you clarify the expected time of advancement in the drop-off time for a passenger when they are assigned to vehicle 3?''; 
    \[ viod(tp(3), eta(3)) \]
    \item ``What is the expected rate of delay for picking up the passenger when traveling in vehicle 1?''; 
    \[ pctd(tp(1), eta(1)) \]
    \item ``What is the expected rate of delay for dropping off the passenger when traveling in vehicle 1?''; 
    \[ pctd(td(1), eta(1)) \]
    \item ``How likely is it that the passenger will be picked up ahead of schedule in vehicle 1?''; 
    \[ pcta(tp(1), eta(1)) \]
    \item ``How likely is it that the passenger will reach their destination ahead of schedule in vehicle 1?''; 
    \[ pcta(td(1), eta(1)) \]
    \item ``What factors lead to delays when a passenger is assigned to vehicle 1?''; 
    \[ sp(0,1); sd(0,1) \]
    \item ``What were the reasons for choosing vehicle 2 over vehicle 3 for this assignment?''; 
    \[
    \begin{aligned}
    vcv(C(3), O(1,3)); \\
    \Phi3(r(2), r(3)); \Phi3(rd1(2), rd1(3)); \Phi3(rd2(2), rd2(3))
    \end{aligned}
    \]
    \item ``What led to the algorithm's decision to overlook vehicle 1?''; 
    \[ vcv(C(1), O(1,1)) \]
    \item ``How does vehicle 1 outperform vehicle 2 when capacity constraints are not a factor?''; 
    \[
    \begin{aligned}
    \Phi1(vioa(tp(1), eta(1)), vioa(tp(2), eta(2))); \\
    \Phi1(vioa(td(1), eta(1)), vioa(td(2), eta(2))); \\
    \Phi1(viod(tp(1), eta(1)), viod(tp(2), eta(2))); \\
    \Phi1(viod(td(1), eta(1)), viod(td(2), eta(2))); \\
    \Phi4(sp(0,1), sp(0,2)); \Phi4(sd(0,1), sd(0,2))
    \end{aligned}
    \]
    \item ``Is vehicle 1 more successful at minimizing time violations compared to vehicle 2?''; 
    \[
    \begin{aligned}
    \Phi1(vioa(tp(1), eta(1)), vioa(tp(2), eta(2))); \\
    \Phi1(vioa(td(1), eta(1)), vioa(td(2), eta(2))); \\
    \Phi1(viod(tp(1), eta(1)), viod(tp(2), eta(2))); \\
    \Phi1(viod(td(1), eta(1)), viod(td(2), eta(2)))
    \end{aligned}
    \]
    \item ``Does vehicle 1 offer a route with fewer stops than vehicle 2?''; 
    \[
    \Phi4(sp(0,1), sp(0,2)); \Phi4(sd(0,1), sd(0,2))
    \]
    \item ``Is there a possibility of a delay for the passenger if they are assigned to vehicle 3?''; 
    \[
    viod(tp(3), eta(3)); viod(td(3), eta(3))
    \]
    \item ``Is it possible that the passenger will arrive earlier than expected if assigned to vehicle 3?''; 
    \[
    vioa(tp(3), eta(3)); vioa(td(3), eta(3))
    \]
    \item ``What is the difference in reward when the passenger is assigned to vehicle 1 versus vehicle 2?''; 
    \[
    \Phi3(r(1), r(2)); \Phi3(rd1(1), rd1(2)); \Phi3(rd2(1), rd2(2))
    \]
    \item ``Why was vehicle 1 chosen for the passenger's assignment?''; 
    \[
    vcv(C(1), O(1,1)); r(1); rd1(1); rd2(1)
    \]
    \item ``Which vehicle is scheduled to pick up the passenger?''; 
    \[ car(1) \]
    \item ``How many vehicles are available right now to pick up the passenger?''; 
    \[ availablecar(1) \]
\end{enumerate}

\paragraph{Category 2}
\begin{enumerate}
    \item ``What are the potential consequences of placing the passenger in alternative vehicle 1?''; 
    \[ search(1) \]
    \item ``What does occur when traffic becomes congested?''; 
    \[ cong(0) \]
    \item ``What happens if vehicle 1 breaks down?''; 
    \[ exclude(1) \]
    \item ``What should we do if this trip includes 2 passengers?''; 
    \[ multi(2) \]
    \item ``What is the reassignment plan for passengers currently on vehicle 2 if it breaks down?''; 
    \[ reassign(2) \]
\end{enumerate}

\subsection{Additional User Feedback}

\paragraph{Selected Positive Feedback} 
\begin{itemize}
    \item ``The chatbot explainer makes it much easier to understand because I can formulate any specific doubts I have and the chatbot can address them directly in order for me to actually understand the algorithm and why it chose a specific vehicle over another.''
    \item ``I can understand the essential logics of this prompt, the system is capable to response complex question as well.''
    \item ``I think this version of explanation makes more sense and much more clear then previous two. User has more flexibility and less restriction to ask question regarding different aspects. The answer towards the question will be more straightforward and understandable. All the information provided in this pattern will be more comprehensive.''
    \item ``This explanation helps me understand more background info, which I didn't have or missed in the previous two setups. Although the waiting time is a bit long (adding a simple gif while waiting might help lower the latency?), overall it reacts within a tolerable time. ''
    \item ``It can perfectly answer the suggested questions. It can also provide a reasonable answer for some general questions. It helped me to understand the algorithm better. The check box styled question and answer also helped me understand the algorithm since they provide detailed and specific examples.''
    \item ``It can perfectly answer the suggested questions. It can also provide a reasonable answer for some general questions. It helped me to understand the algorithm better. The check box styled question and answer also helped me understand the algorithm since they provide detailed and specific examples.'' 
\end{itemize}

\paragraph{Selected Critical Feedback}
\begin{itemize}
    \item ``I think that this provides great in-depth explanations but many general users wouldn't love to wait 30 seconds for a generated response. I suppose it is a balance, but it also requires users to have the right questions to ask.''
    \item ``Some responses were very slow. System crashed on initial try.''
    \item ``I have another feedback but I do not think it is a big problem right now. The amount of time that the AI chat bot takes is too long.''
    \item ``I had to phrase my question in a specific way. I got lucky that it popped up.''
    \item `` `The estimated time of arrival for the passenger if they were to be assigned to vehicle 3 is 17 minutes for pick-up and 28 minutes for drop-off.' This seems misleading, if I had not asked what time the passenger's requested pickup time was I would not know what time the estimated pickup and dropoff is (assuming 4:15 + 17 minutes for pickup?) And the dropoff time is unknown, I do not know the travel time etc. The delay question response seems like it only considers delay due to extra stops. Can it include delay due to travel time?'' 
    \item ``When I asked `which vehicle will take over the passengers if vehicle 3 breaks down the bot said “there is no vehicle assigned to take over the passengers' but when I asked `what will happen if vehicle 3 becomes inoperable', the bot said `the trip will be assigned to vehicle 0.' Is there a difference between breaking down and being inoperable that causes the results to be different?'' 
\end{itemize}

\begin{figure*}[t]
\centering
  \includegraphics[width=\linewidth]{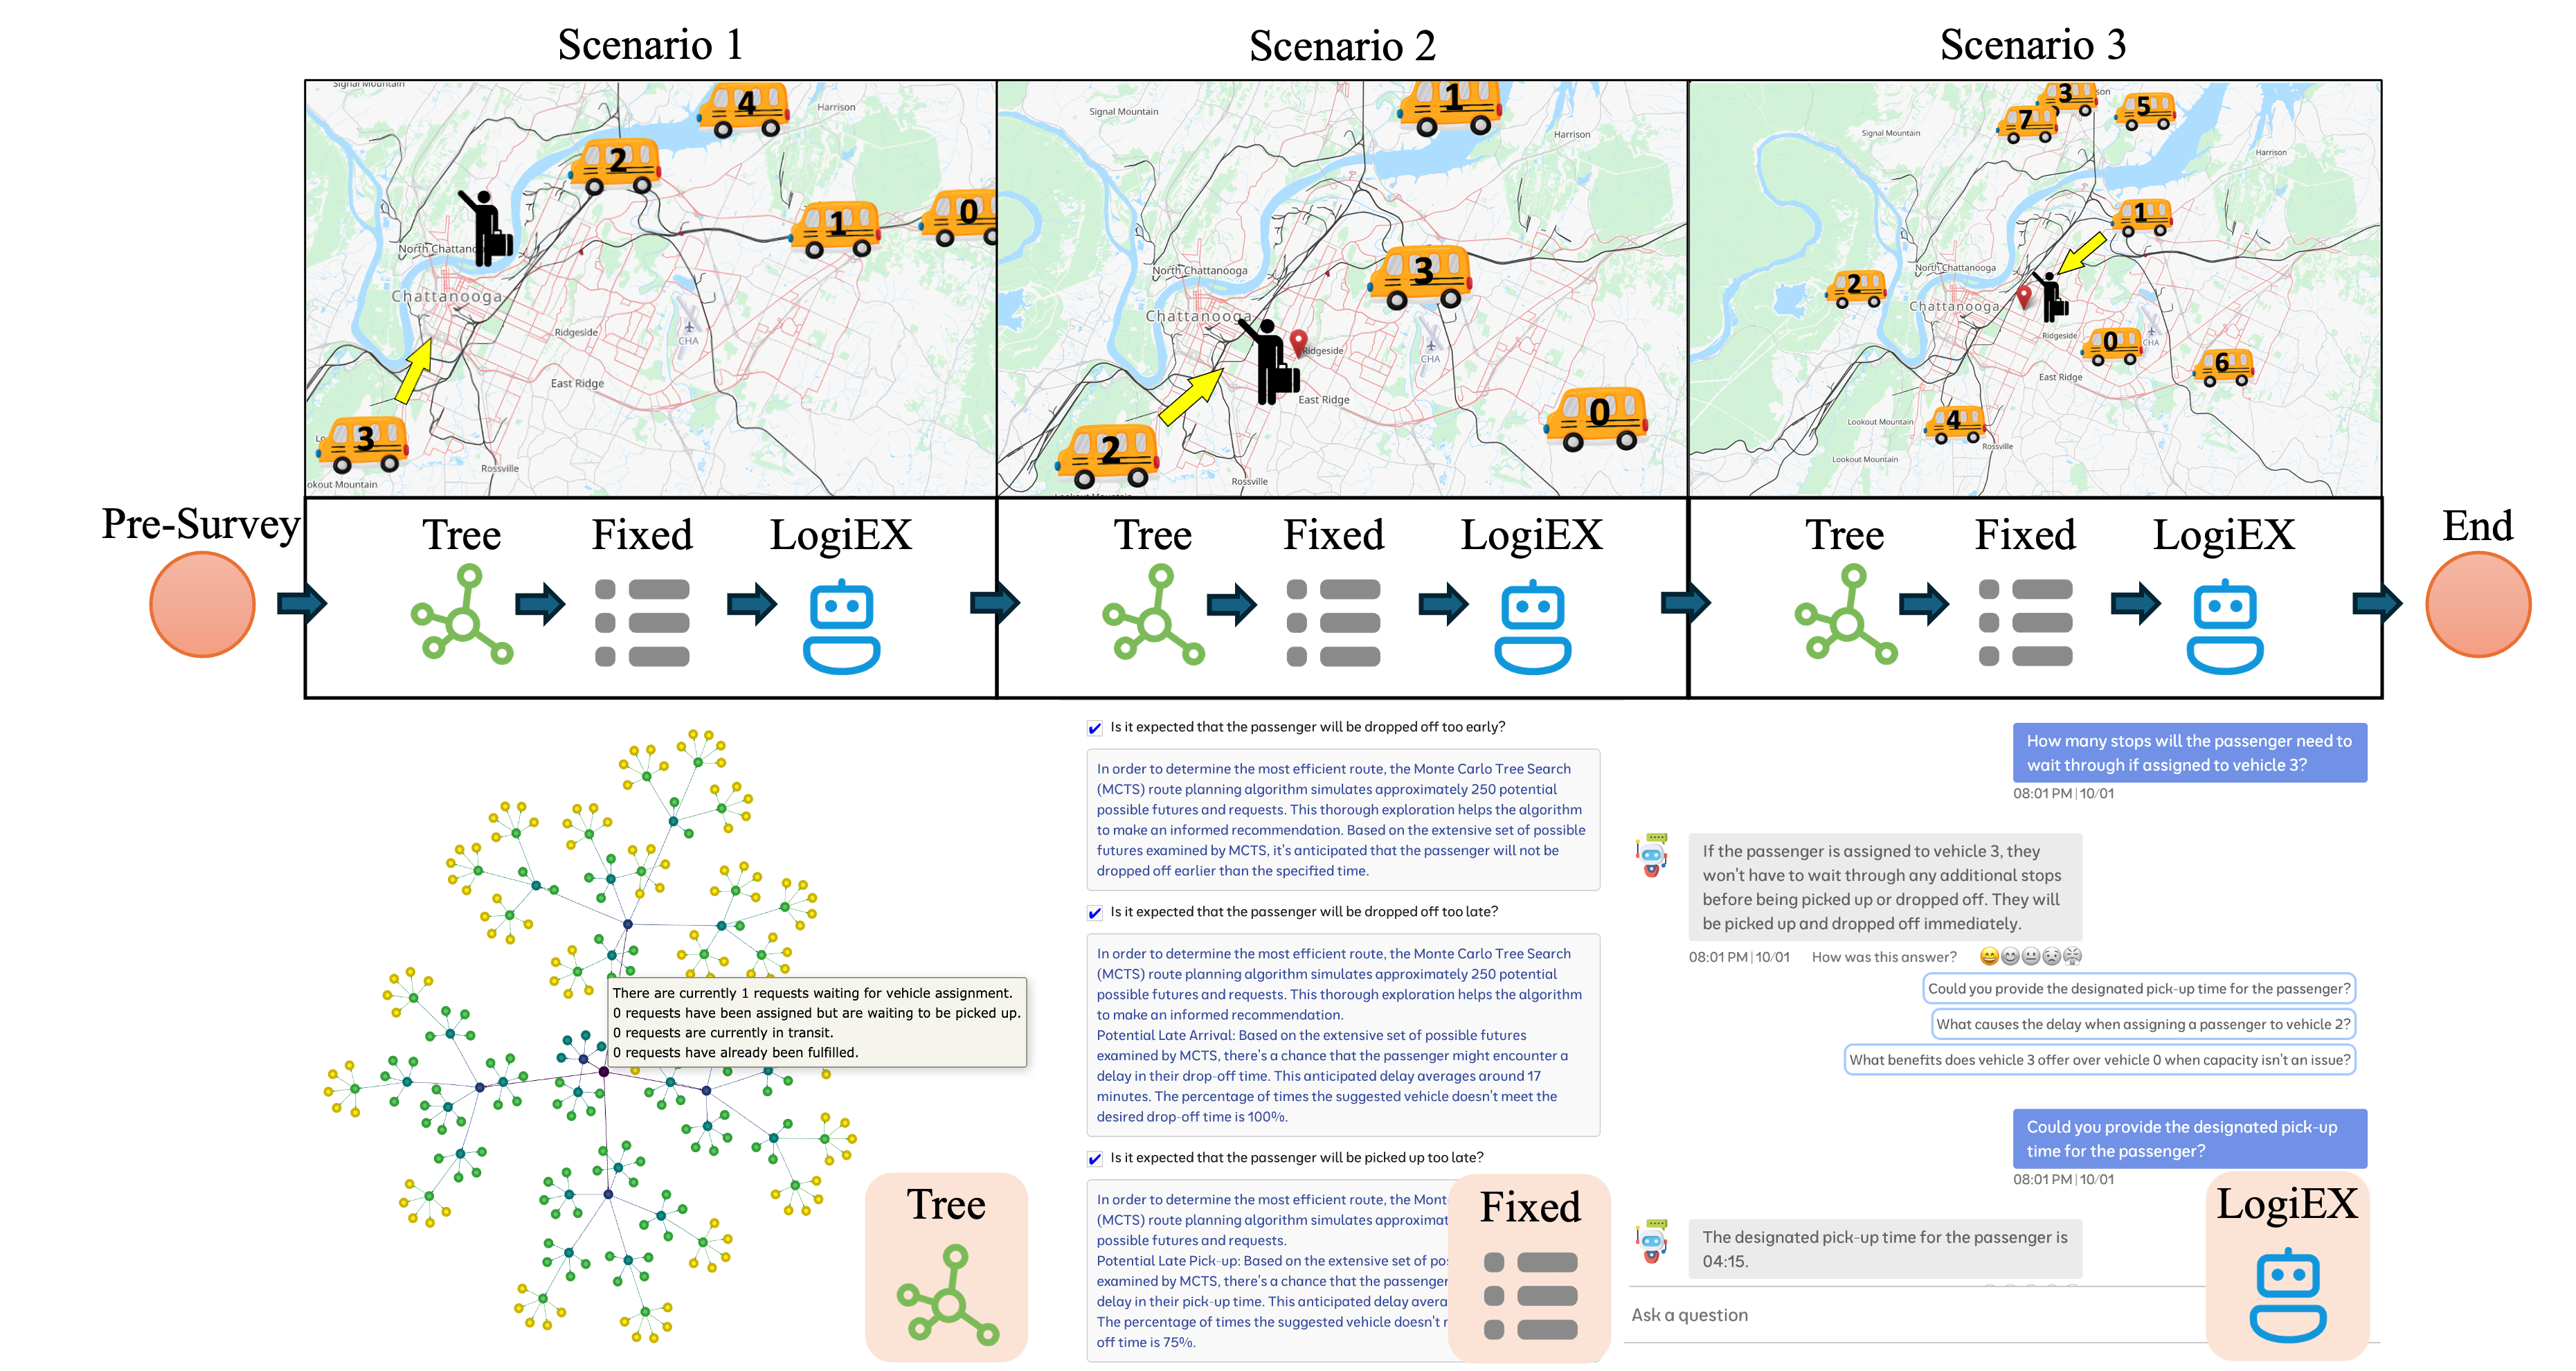}
  \caption{Survey Procedure.}
  \label{fig:interface}
\end{figure*}

\begin{figure*}[t]
\centering
  \includegraphics[width=\linewidth]{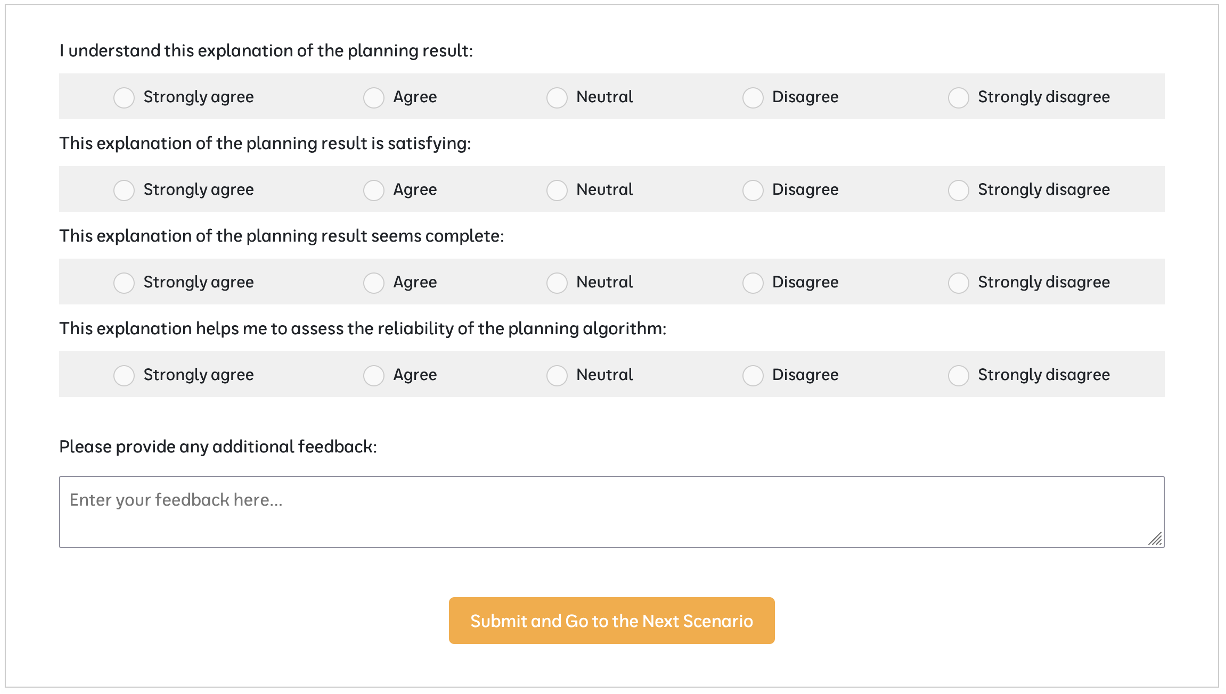}
  \caption{Survey Rating System Interface.}
  \label{fig:interface}
\end{figure*}

\begin{table}[t]
\centering
    \scriptsize
    \caption{Accuracy in Generating the Correct Logic.}
    \begin{tabular}{l|c|c|c}
    \toprule
      \textbf{Question Type} & \textbf{Model} & \textbf{Acc$@$1} & \textbf{Acc$@$3} \\
      \midrule
      1  &  GPT-4 & 100\% & 100\% \\
    \midrule
    2  &  GPT-4 & 100\% & 100\% \\
    \midrule
    3  &  GPT-4 & 100\% & 100\% \\
    \midrule
    4  & GPT-4 &  85\%  &  85\% \\
    \midrule
    5  & GPT-4 &  100\%  &  100\%\\
    \midrule
    6  & GPT-4 &  100\% & 100\% \\
    \midrule
    7  & GPT-4 & 100\% & 100\% \\
    \midrule
    8  & GPT-4 & 100\% & 100\% \\
    \midrule
    9  & GPT-4& 100\% & 100\% \\
    \midrule
    10  &  GPT-4 & 100\% &  100\%\\
    \midrule
    11  &  GPT-4 & 100\% & 100\% \\
    \midrule
    12  &  GPT-4 & 100\% & 100\% \\
    \midrule
    13  & GPT-4 & 100\% &  100\%\\
    \midrule
    14  & GPT-4 & 100\% & 100\% \\
    \midrule
    15  & GPT-4 &  100\%  & 100\% \\
    \midrule
    16  & GPT-4 & 100\% & 100\% \\
    \midrule
    17  & GPT-4 & 100\% & 100\% \\
    \midrule
    18  & GPT-4& 100\% & 100\% \\
    \midrule
    19  &  GPT-4 & 100\% & 100\% \\
    \midrule
    20  &  GPT-4 & 100\% & 100\% \\
    \midrule
    21  &  GPT-4 & 100\% & 100\% \\
    \midrule
    22  & GPT-4 &  100\%  & 100\% \\
    \midrule
    23  & GPT-4 &  100\%  & 100\% \\
    \midrule
    24  & GPT-4 &  100\%  & 100\% \\
    \midrule
    25  & GPT-4 & 100\% & 100\% \\
    \midrule
    26  & GPT-4 & 100\% &  100\%\\
    \midrule
    27  & GPT-4& 100\% & 100\% \\
    \midrule
    28  & GPT-4& 95\% & 95\% \\
    \midrule
    29  &  GPT-4 & 100\% & 100\% \\
    \midrule
    30  &  GPT-4 & 100\% & 100\% \\
    \midrule
    31  &  GPT-4 & 100\% & 100\% \\
    \midrule
    Overall  & GPT-4 & 99.35\% & 99.35\% \\
    \bottomrule
    \end{tabular}
     \label{tab:economy}
\end{table}

\begin{table}[t]
\centering
    \scriptsize
    \caption{Accuracy in Generating the Correct Logic.}
    \begin{tabular}{l|c|c|c}
    \toprule
      \textbf{Question Type} & \textbf{Model} & \textbf{Acc$@$1} & \textbf{Acc$@$3} \\
      \midrule
    Base-Level Evidence  & LogiEx (w/ GPT-4) & 100.0\% &  100.0\% \\
    \midrule
    Derived Evidence  &  LogiEx (w/ GPT-4) & 99.21\% &  99.21\%  \\
    \midrule
    Logic Comparison Evidence  &  LogiEx (w/ GPT-4) & 98.75\% &  98.75\%  \\
    \midrule
    Overall  & LogiEx (w/ GPT-4) & 99.35\% & 99.35\% \\
    \bottomrule
    \end{tabular}
     \label{tab:logic}
\end{table}

\begin{table}[t]
\centering
    \scriptsize
    \caption{Accuracy in Classifying Query Types.}
    \begin{tabular}{l|c|c}
    \toprule
    \textbf{Question Type} & \textbf{LogiEx (w/ GPT-4) Acc$@$3} & \textbf{BERT Acc$@$3} \\
    \midrule
    Base-Level Evidence &  98.75\% & 99.38\% \\
    \midrule
    Derived Evidence  &  93.68\% &  90.00\% \\
    \midrule
    Logic Comparison Evidence  &  100.0\% &  98.75\% \\
    \midrule
    Overall  & 95.81\% &  93.55\% \\
    \bottomrule
    \end{tabular}
    \label{tab:classify}
\end{table}
